# Supplementary material for: Tree pyramidal adaptive importance sampling
Source: arXiv:1912.08434 source file (2020-03-23)
Supplement: Supplementary file 1 [file evidence_approx.tex]

The Tree Pyramid sampling approach partitions the space in hierarchical non-uniform convex hyper-volumes. This lets us compute the evidence by summation of each sample probability mass. First, we approximate the probability density inside each partition hyper-volume to be uniform, the evidence of the sampled posterior density function is thus approximated by:

$$ Z = \sum_{i=0}^N P(c_i|D)r_i^k,$$

where each discrete piece of evidence $Z_i$ is obtained by computing the probability mass contained in each hyper-volume using the sample radius $r_i$ and its likelihood value $P(c_i | D)$. Figure~\ref{fig:evidence_approximation} shows several examples of the evidence computed on a 1-D example with different posterior distributions and number of samples. This approximation relaxes the intractability problem of evidence computation for Bayesian inference applications and allows the computation of normalized probabilities.

\begin{figure}
    \centering
    \includegraphics[width=0.32\textwidth]{figures/evidence_approx_1.png}
    \includegraphics[width=0.32\textwidth]{figures/evidence_approx_2.png}
    \includegraphics[width=0.32\textwidth]{figures/evidence_approx_3.png}
    \caption{Evidence approximation on three different PDFs. The sampling space is bounded to [-1,1]. Left: A 1-D normal distribution with $\mu=0$ $\sigma=0.1$ approximated by 20 samples. Middle: A 1-D gaussian mixture model with $\mu=[0.4 -0.2]$ $\sigma=[0.01, 0.3]$ approximated by 100 samples. Right: A 1-D gaussian mixture model with $\mu=[0.4 -0.2]$ $\sigma=[0.01, 0.3]$ approximated by 100 samples.}
    \label{fig:evidence_approximation}
\end{figure}
