# Supplementary material for: Tree pyramidal adaptive importance sampling
Source: arXiv:1912.08434 source file (2020-03-23)
Supplement: Supplementary file 2 [file pdf_approximation.tex]

\subsection{PDF Approximation}
The result of a sampling algorithm is a set of samples drawn from the target PDF, a byproduct of AIS methods is the adapted proposal distribution. We evaluate how close to the true distribution the adapted proposal is, for MCMC algorithms we use a KDE approximation from the samples. For the continuous PDF fitting, two methods are used: Kernel Density Estimation and Nearest Neighbor Approximation. Figure~\ref{fig:PDF_approximation} shows an example of the two approximation methods on a bi-variate Gaussian mixture model distribution.

\subsubsection*{Kernel Density Estimation}
KDE is a well known method used to estimate an unknown PDF from its drawn samples \cite{Epanechnikov69}. Consider $\mathcal{X} = {x_0, \dots ,x_n }$ a set of samples drawn from an unknown PDF $P$, its Kernel Density Estimator $\hat{P}$ is
    $$\hat{P}(x) = \frac{1}{nh} \sum^{n-1}_{i=0} K\Big( \frac{x - x_i}{h} \Big),$$
where $K$ is a kernel function and $h$ is a smoothing parameter a.k.a. \textit{bandwidth}. For discussion about kernel and bandwidth selection criteria we refer the reader to \cite{jones96}. In this paper, we have used a Gaussian kernel function and manually tuned $h$ to fit the ground truth distribution. All the sampling methods compared in this paper use the same KDE kernel and bandwidth to obtain the sample-based PDF approximation.

\subsubsection*{Nearest Neighbor Approximation}
\todo[inline]{Explain how to normalize this approximation such that it integrates to 1 or why we can use it as is without needing to normalize.}
Unfortunately, the computational cost of computing the esimated density using a KDE estimator is $\mathcal{O}(N)$. In the evaluation process we consider both small and big sample sets, especially for the performance evaluation in higher dimensions. As an alternative to KDE we use a computationally tractable approximation function such as the nearest neighbor approximation with $\mathcal{O}(log(N))$ cost defined by:
$\hat{P}(x) = P(\mathcal{X}[argmin_i(||x-x_i||)])$.

\begin{figure}
    \centering
    \includegraphics[width=0.99\textwidth]{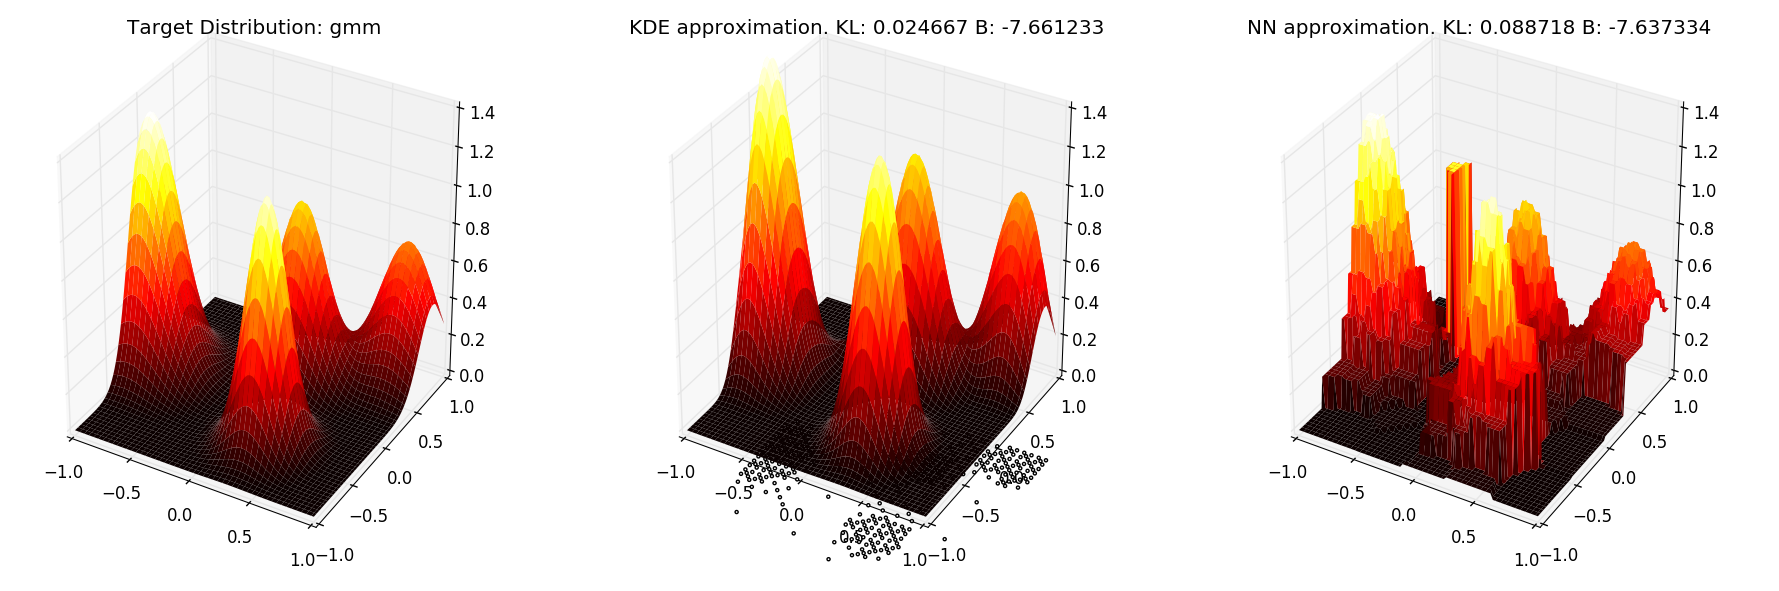}
    \caption{Example of the PDFs approximation methods used for the experimental comparison with their corresponding similarity metrics. Right: Ground truth distribution, a Bi-variate Gaussian Mixture Model. Middle: Samples (obtained with our TP method) and its Kernel Density Estimate approximation with bandwidth = 0.02. Left: Nearest neighbor approximation.}
    \label{fig:PDF_approximation}
\end{figure}
