# Supplementary material for: Tree pyramidal adaptive importance sampling
Source: arXiv:1912.08434 source file (2020-03-23)
Supplement: Supplementary file 3 [file sampling_methods.tex]

\todo{Comment on general importance sampling and the relation of the importance weight to the evaluated sampling methods.}

\todo{Elaborate on the reasons to select the different sampling methods by commenting on their strengths and weaknesses.}

\subsubsection{Rejection Sampling}

\subsubsection{Uniform Importance Sampling}
- Simulated annealing

\subsubsection{Markov Chain Monte Carlo}
\paragraph{Metropolis-Hastings}

\paragraph{Hybrid Monte Carlo}

\subsubsection{Nested Sampling}
\todo{Comment on the nested sampling approach, its variations and the reason to use Multi-Nested Sampling.}

\section*{On sampling methods, thoughts and discussion}
The process of sampling consists on obtaining a subset of elements that are representative of a broader set. For the subset to be representative, it has to preserve the statistical properties of the super-set that it is representing. For example, imagine a city with a population of 10000 people and we're interested in their age (sample space). In the discrete case, simply sampling at random from the population is a good strategy to generate a subset that is representative. However, sometimes super-sets are continuous (have infinite elements) and are described by a probability density function (PDF). Generating samples from a continuous PDF is solved for Normal distributions using the Box-Mueller transform, the inverse distribution function or less efficiently using the central limit theorem. However if the PDF is complex, non-parametric or simply unknown we need other approaches to generate samples from it. In these cases is where other sampling techniques such as Importance Sampling, Simulated annealing, MCMC and so on become useful. Later, the samples can be used to build an approximation of the continuous PDF (e.g. using Kernel Density Estimation) that can be used to make inference about modes, mean, entropy, intervals etc.
