# Supplementary material for: Tree pyramidal adaptive importance sampling
Source: arXiv:1912.08434 source file (2020-03-23)
Supplement: Supplementary file 4 [file applications.tex]

\subsection{Object pose inference from depth images}

\subsection{Macro-molecular ligand-receptor docking}
Protein–protein interactions are involved in virtually all cellular processes, such as protein expression regulation, cell-cycle control or immune response, among many others (Eisenberg et al., 2000). Characterizing such interactions at atomic level is of paramount importance to better understand pathological conditions at molecular level.
\begin{itemize}
    \item Metrics: minimum energy, gibbs free energy
    \item Sota techniques: GSO sampling. PSO. 
    \item Score functions: Anisotropic Network Model allows certain flexibility in ligand and receptor. Adds about 20 dimensions to the problem. Force-field approaches. Free-energy computations.
    \item Interesting problem ADN - enzyme
\end{itemize}
